# Supplementary material for: Circular-Symmetric Correlation Layer based on FFT
Source: arXiv:2107.12480 source file (2021-07-26)
Supplement: Supplementary file 1 [file appendix.tex]

{\centering
{\LARGE\bf Supplementary Material\par}
}
\setcounter{section}{0}

\section{Background on Group Theory}
The formalism used in the paper is based on various concepts in group theory and abstract algebra. In this part, we aim to provide this key concepts, and their corresponding notations and definitions.

\paragraph{Group:} A group $\mathcal{G}$ is a set which is equipped with a binary operation and  has the following
properties: 
\begin{itemize}
    \item $\mathcal{G}$ is closed under its binary operation;
    \item the group operation is associative –i.e., (g1g2)g3 = g1(g2g3)¦g1; g2; g3 > G;
    \item there exists an identity e > G such that ge = eg = g and ;
    \item every element g > G has an inverse g−1 > G, such that gg−1 = g−1g = e.
\end{itemize}
\paragraph{Subgroup:}  A subset H b G is a subgroup of G (G B H) iff H equipped with
the binary operation of G forms a group. Moreover, if H is
a proper subset of G, H is a proper subgroup of G, H < G.
Two groups are isomorphic G  H if there exists a bijection
  G �� H, such that g1g2 = g3  (g1)(g2) =
(g3)¦g1; g2; g3. If this last relation holds for a surjective
mapping (not necessarily one-to-one) then  is a homomorphic
mapping and H is isomorphic to a subgroup of G.
Cayley Diagram. The set A b G is called the generating

 Give a group $G$ and a normal subgroup $H\mathrel{\lhd}G$, there is an

 \paragraph{Group action:} We are interested on the way a group “acts” on the input
and output of a deep network. Function $\gamma:\mathcal{G}\times\mathbb{X}\to \mathbb{X}$ is the left action of group $\mathcal{G}$ on $\mathbf{x}$ iff I) 
$\gamma(e,\mathbf{x}) = \mathbf{x}$ and; II)$\gamma(g_1,\gamma(g_2,\mathbf{x})) = \gamma(g_1g_2,\mathbf{x})$

\paragraph{Action on the indices:} Lets $\mathbf{x}= [x_1,\dots,x_N] \in \mathbb{X}^N$ be a vector of N variables taking value in domain $\mathbb{X}$. $\mathbb{N} = \{1,\dots,N\}$ denotes the indices of $\mathbf{x} = \left(x_n\right)_{n\in\mathbb{N}}$. The action of $g$ on a vector/sequence $\overrightarrow{\mathbb{N}} = \{1,\dots,N\}$  is defined similarly
$g\overrightarrow{\mathbb{N}} = \{g1,\dots,gN\}$. Considering this, the $\mathcal{G}$-action on $\mathbf{x}= [x_1,\dots,x_N]$ is $g\mathbf{x}= [x_{g1},\dots,x_{gN}]$.

\paragraph{Faithful $\mathcal{G}$-action:} $\mathcal{G}$-action is faithful iff two groups are isomorphic $\mathcal{G}\cong \mathcal{G}_{\mathbb{N}}$.

\paragraph{Normal subgroup:} Let $H$ be a subgroup of a group $G$. The similarity transformation of $H$ by a fixed element $x$ in $G$ not in $H$ always gives a subgroup. If 
\[
xHx^{-1} = H
\]
for every element $x$ in $G$, then $H$ is said to be a normal subgroup of G, written $H \lhd G$ (Arfken 1985, p. 242; Scott 1987, p. 25). Normal subgroups are also known as invariant subgroups or self-conjugate subgroup (Arfken 1985, p. 242).

\paragraph{Orbits:} Given $\mathcal{G}$-action on $N$, the orbit of $n \in N$ is all the members to which it can be moved, $\mathcal{G}n = \{gn \mid n \in N\}$.

\paragraph{Relation:} A relation from a set A to a set B is a subset of A;times;B. Hence, a relation R consists of ordered pairs (a,b), where ;isin;A and bamp;isin;B. If (a,b)amp;isin;R, we say that is related to.

\paragraph{Subdirect product:}

\paragraph{regularity:} The group action is free or semi-regular iff
¦n1;n2 > N, there is at most one g > G such at
gn1 = n2, and the action is regular iff it is both transitive
and free – i.e., for any pair n1;n2 > N, there is
uniquely one g > G such that gn1 = n2. Any free action
is also faithful. We use a similar terminology for
GN. That is we call GN semi-regular iff ¦n1;n2 > N at most one gN > GN moves n1 to n2 and GN is regular if
this number is exactly one.

\paragraph{Group action:} $\g{G}$-action on $\mathbb{N}$, denoted as $\g{G}_{\mathbb{N}}$ ($\g{G}_{\mathbb{N}}\leq \g{G}$), captures the structure of $\g{G}$ when it acts on $\mathbb{N}$. We use $g_{\mathbb{N}}$ to denote the image of $g$

\paragraph{Cyclic Group:}
\paragraph{Isomorphic:}\gls{isomorphic}
\paragraph{\Gls{subdir}:}
\paragraph{Powerset of the set $S$:}It is denoted as $\wp(S)$ or $2^{S}$
\paragraph{binary \glspl{relation}}
\paragraph{Homogeneous Space and Transitivity:} Transitivity is the property that taking any $x_0 \in \mathcal{X}$, any other $x\in \mathcal{X}$ can be reached by the action of some $g \in G$, i.e., $x= g(x_0)$. If the action of $G$ on $\mathcal{X}$ is \gls{transitive},
we say that $X$ is a \gls{homogeneous space} of $G$.
\paragraph{Automorphism:}

\section{Definitions}

\begin{tcolorbox}[
colback=gray!20!white,
colframe=gray!30!white,
coltitle=black,
title={\textbf{Homogeneous space $\mathcal{X}$}}
]
\begin{definition}
\textup{
If taking any $x_0 \in X$, any other $x \in \mathcal{X}$ can be reached
by the action of some $g \in G$, i.e., $x = g(x_0)$. This property
is called \textbf{transitivity}, and if the action of $G$ on $\mathcal{X}$ is transitive, we say that $\mathcal{X}$ is a \textbf{homogeneous space} of $G$.
}
\label{def:homo}
\end{definition}
\end{tcolorbox}

\begin{tcolorbox}[
colback=gray!20!white,
colframe=gray!30!white,
coltitle=black,
title={\textbf{symmetry}}
]
\begin{definition}
\textup{
A symmetry is a set of transformations applied to a structure, such that the transformations preserve the properties of the structure. Generally it is also presumed that the transformations must be invertible, i.e. for each transformation there is another transformation, called its inverse, which reverses its effect.}
\par\noindent\textup{Symmetry is thus mathematized as an operator acting on an object, where the defining feature is that the object remains unaltered. Expressed in other words, the object is invariant under the symmetry transformation.
}
\label{def:sym}
\end{definition}
\end{tcolorbox}

\begin{tcolorbox}[
colback=gray!20!white,
colframe=gray!30!white,
coltitle=black,
title={\textbf{Normal subgroups}}
]
\begin{definition}
\textup{
a
}
\label{def:norm}
\end{definition}
\end{tcolorbox}

\section{Code, Datasets, and Experimental Settings}

\subsection{Creation of Dataset}
\begin{table}[!ht]
\caption{Network architectures. CCL$($c$_\textsc{out})$: c$_\textsc{out}$ implies number of output channels. $\text{FC}(l_\textsc{in}, l_\textsc{out})$: $l_\textsc{in}$ and $l_\textsc{in}$ imply input and output features dimensions, respectively. $\text{MaxPool}(k, s)$: $k$ and $s$ imply kernel and stride sizes, respectively.
$\text{AvgPool}(k)$: $k$ implies kernel sizes. $\text{BN}$ denotes batch normalization. Note that the global average pooling makes the network invariant to the input roll.
}
\centering
{\small
\setlength\tabcolsep{9pt}
\begin{tabular}{c|c|c|c}
\toprule
\backslashbox{Layer}{Dataset} &
MNIST
& CIFAR10 &
Panoramic ShapeNet
\\
\midrule
Input
& $f\in \mathbb{R}^{1\times 28\times28}$
& $f\in \mathbb{R}^{3\times 32\times32}$
& $f\in \mathbb{R}^{1\times 48\times100}$
\\ 
\midrule
1
& \text{CCL(8), ReLU}
& \text{CCL(128), ReLU}
& \text{CCL(64), BN, ReLU}
\\
2
& \text{CCL(8), ReLU}
& \text{CCL(128), ReLU}
& \text{MaxPool(2, 2)}
\\
3
& \text{MaxPool(2, 2)}
& \text{MaxPool(2, 2)}
& \text{CCL(64), BN, ReLU}
\\
4
& \text{CCL(8), ReLU}
& \text{CCL(128), ReLU}
& \text{CCL(128), BN, ReLU}
\\
5
& \text{CCL(8), ReLU}
& \text{CCL(256), ReLU}
& \text{MaxPool(2, 2)}
\\
5
& \text{MaxPool(2, 2)}
& \text{MaxPool(2, 2)}
& \text{CCL(256), BN, ReLU}
\\
6
& \text{CCL(10), ReLU}
& \text{AvgPool(8)}
& \text{AvgPool(300)}
\\
7
& \text{AvgPool(7), Softmax}
& \text{FC(256, 120), ReLU}
& \text{FC(256, 100), ReLU}
\\
8
& 
& \text{FC(120, 84), ReLU}
& \text{FC(100, 55), Softmax}
\\
9
&
& \text{FC(84, 10), Softmax}
&
\\
\bottomrule
\multicolumn{4}{l}{\small For regular CNN, the CCL layers are replaced with Conv2d layers.}
\end{tabular}
}
\label{tb:supp}
\end{table}

\subsection{Code and Computational Resources}
We implemented CCL and performed our experiemnts in PyTorch v1.8 \citep{paszke2017automatic} and used the Adam optimizer \citep{kingma2014adam} with learning rate of $0.001$. We initialized all parameters randomly. Each CCL layer has $C_{out}\times C_{in} \times K_1 \times K_2$ parameters similar to that of a CNN layer. The
time complexity for training a CCL layer is $O(C_{in}\times C_{out}\times N \times \log(N))$ per data sample and epoch, where $N$ is the dimension of input data, and the space complexity is $O(b\times C_{in} \times C_{out} \times N)$ where $b$ is the batch size.
We learned and tested all the models on an Intel Core i7 CPU@3.7GHz with 8 GB of RAM. Per-epoch training time varied from $30$ms in smaller datasets to $1.2$ s in larger experiments and $20$ epochs sufficed for most experiments.
